# Supplementary material for: Comparison of Multilingual and Bilingual Models for Satirical News Detection of Arabic and English
Source: arXiv:2411.10730 source file (2024-11-16)
Supplement: Supplementary file 1 [file appendix.tex]

\appendix

\addappheadtotoc
\setboolean{@twoside}{false}
\appendixpage

% \chapter{Lists}
\addcontentsline{toc}{section}{List of Abbreviations}
\begin{acronym}[\hspace{3cm}]
  \acro{ml}[ML]{Machine Learning}
  \acro{ai}[AI]{Artificial Intelligence}
  \acro{nlp}[NLP]{Natural Language Processing}
  \acro{llm}[LLM]{Large Language Model}
  \acro{llms}[LLMs]{Large Language Models}
  \acro{vlprompt}[VLPrompt]{Variational-autoencoder-Like Prompt}
  \acro{cot}[COT]{Chain-Of-Thought}
  \acro{svm}[SVM]{Support Vector Machine}
  \acro{lstm}[LSTM]{Long Short-Term Memory}
  \acro{cnn}[CNN]{Convolutional Neural Networks}
  \acro{bert}[BERT]{Bidirectional Encoder Representations from Transformers}
  \acro{gpt}[GPT]{Generative Pre-trained Transformer}
  \acro{bow}[BoW]{Bag-of-Words}
  \acro{pos}[POS]{Part-of-Speech}
  \acro{dt}[DT]{Decision Trees}
  \acro{nb}[NB]{Naive Bayes}
  \acro{svc}[SVC]{Support Vector Classifiers}
  \acro{nrg}[NRG]{Narrative Representation Graph}
  \acro{ilp}[ILP]{Integration Linear Program}
  \acro{gru}[GRU]{Gated Recurrent Unit}
  \acro{ela}[ELA]{Error Level Analysis}
  \acro{bns}[BNS]{Bi-Normal Separation}
  \acro{tf-idf}[TF-IDF]{Term Frequency-Inverse Document Frequency}
\end{acronym}
\clearpage
% \listoffigures
% \addcontentsline{toc}{section}{List of Figures}
% \listoftables
% \addcontentsline{toc}{section}{List of Tables}
